# Supplementary material for: PinLanding: Content-First Keyword Landing Page Generation via Multi-Modal AI for Web-Scale Discovery
Source: arXiv:2503.00619 source file (2025-03-01)
Supplement: Supplementary file 1 [file appendix.tex]

\section{This is optional}
